# Supplementary material for: The Ultimate Combo: Boosting Adversarial Example Transferability by Composing Data Augmentations
Source: arXiv:2312.11309 source file (2024-10-23)
Supplement: Supplementary file 1 [file appendix.tex]

\begin{table*}[!htbp]
\scriptsize
\centering

\begin{tabular}{llllllllllll}
\toprule
  \textbf{Model} & \textbf{Attack} & \textbf{Inc-v3}& \textbf{Inc-v4}&\textbf{Res-50}&\textbf{ Res-101}&\textbf{res-152}&\textbf{IncRes-v2}\\ \midrule
  \multirow{5}{*}{Combination-1}
  &\SDTM{}&95.8&\textbf{99.9}&97.1&97.2&97.2&94.5\\
 & \ASDTM{}{}&95.0&99.6&96.1&96.1&96.3&93.4\\
 & \gsdt{}&97.1&\textbf{99.9}&98.4&98.2&98.3&96.6\\
  & \bestcombo{}&\textbf{97.8}&\textbf{99.9}&\textbf{98.8}&\textbf{98.6}&\textbf{98.7}&\textbf{97.7}\\

 \midrule
\bottomrule
\end{tabular}

\caption{\label{tab:table-ens1}Attack success rates (\%) against normally trained models under ensemble-model setting. The combination-1 includes Inc-v4, Res-50,Res-101 and Res-152.}
\end{table*}
